# Supplementary material for: Fill In The Gaps: Model Calibration and Generalization with Synthetic Data
Source: arXiv:2410.10864 source file (2024-10-07)
Supplement: Supplementary file 1 [file Appendix-5.tex]

We present reliability diagrams in our experiments.

TC dataset: 

\begingroup
\setlength{\textfloatsep}{10pt} % Adjust the value as needed

\begin{figure}[h]
\centering
\includegraphics[width=0.5\textwidth]{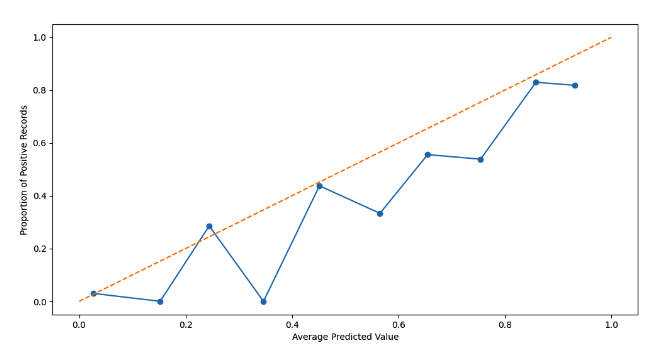}
\caption{\label{fig:bs-tc} The baseline reliability diagram for TC dataset}  
\end{figure}

% \vspace{-10pt} % Adjust the value as needed
\begin{figure}[h]
\begin{subfigure}{0.33\textwidth}
  \includegraphics[width=\linewidth]{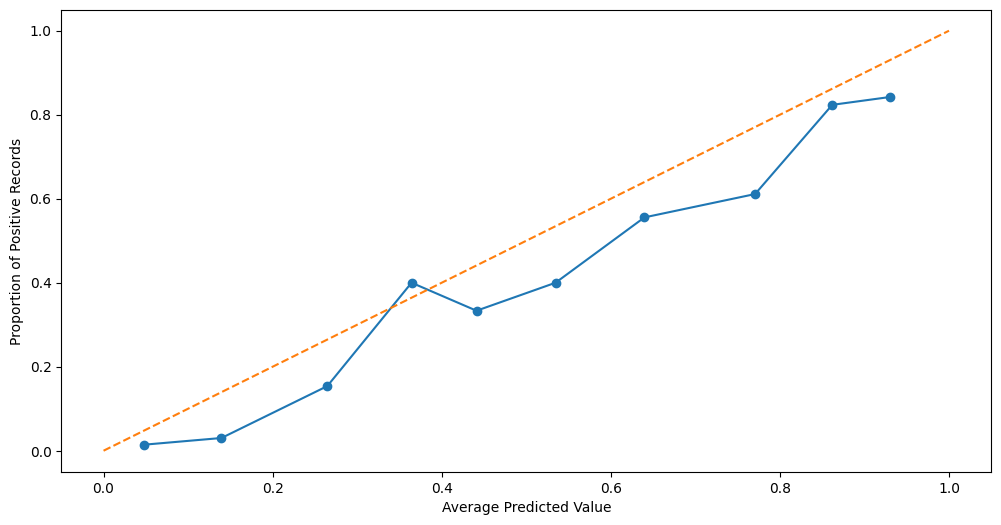}
  \caption{Reliability Diagram of 10 bins}
  \label{fig:rp-10-tc}
\end{subfigure}
\begin{subfigure}{0.33\textwidth}
  \includegraphics[width=\linewidth]{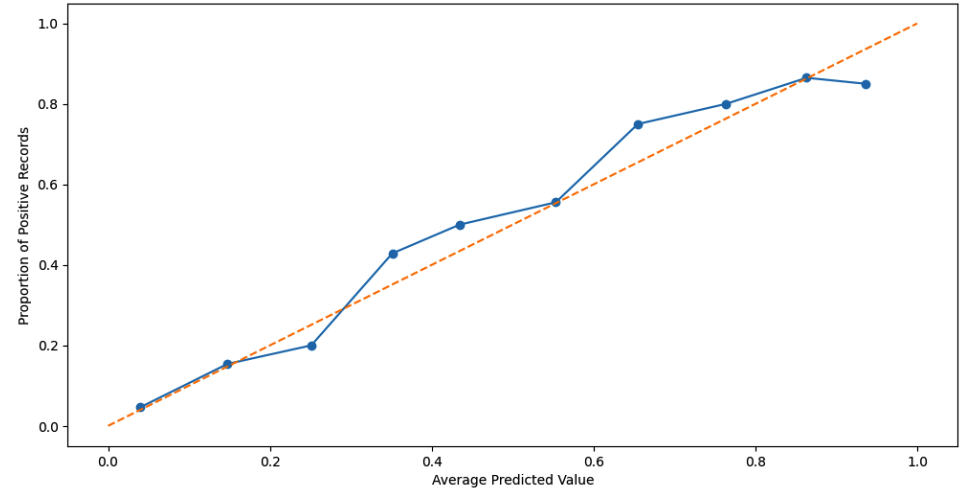}
  \caption{Reliability Diagram of 15 bins}
  \label{fig:rp-15-tc}
\end{subfigure} 
\begin{subfigure}{0.33\textwidth}
  \includegraphics[width=\linewidth]{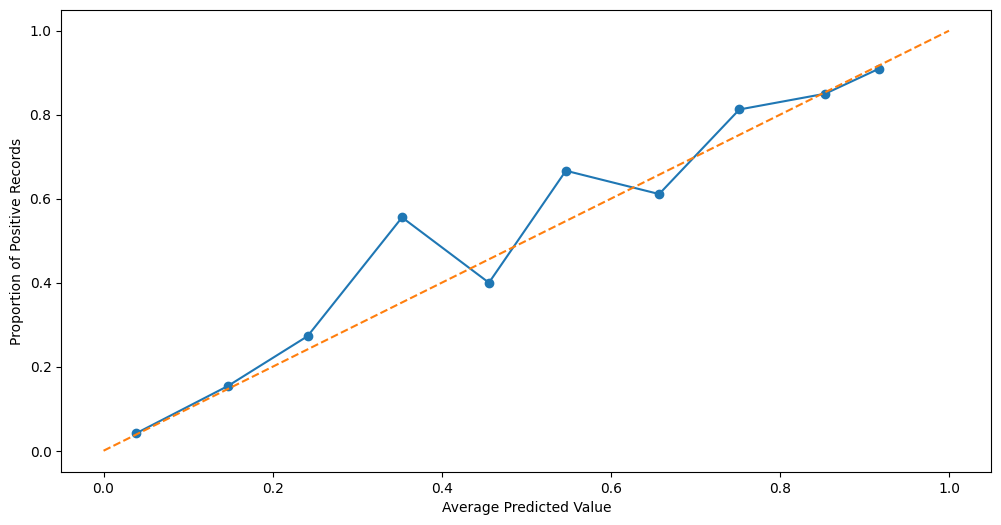}
  \caption{Reliability Diagram of 20 bins}
  \label{fig:rp-20-tc}
\end{subfigure} 
\label{fig:tc-rp}
\caption{Reliability diagrams with synthetic data replacement (synthesis)}
\end{figure}

% \vspace{-50pt} % Adjust the value as needed

\begin{figure}[h]
\begin{subfigure}{0.33\textwidth}
  \includegraphics[width=\linewidth]{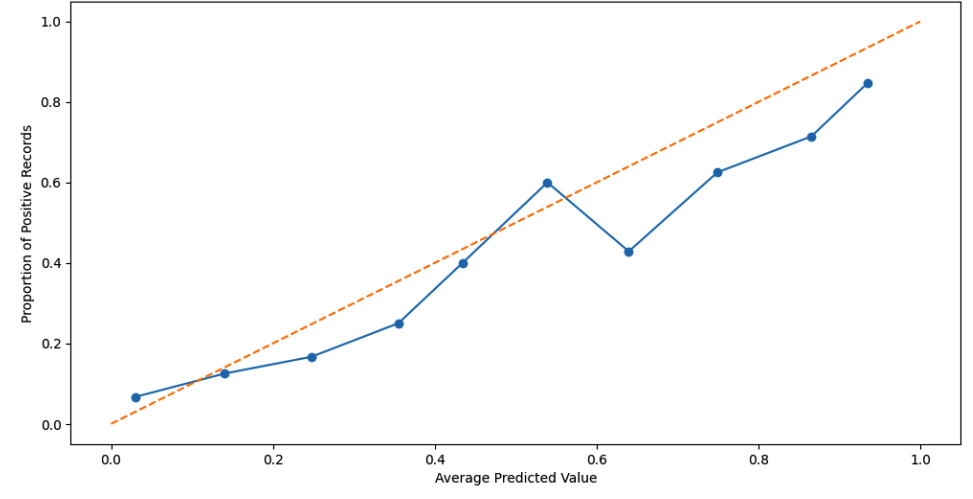}
  \caption{Reliability Diagram of 10 bins}
  \label{fig:ad-10-tc}
\end{subfigure}
\begin{subfigure}{0.33\textwidth}
  \includegraphics[width=\linewidth]{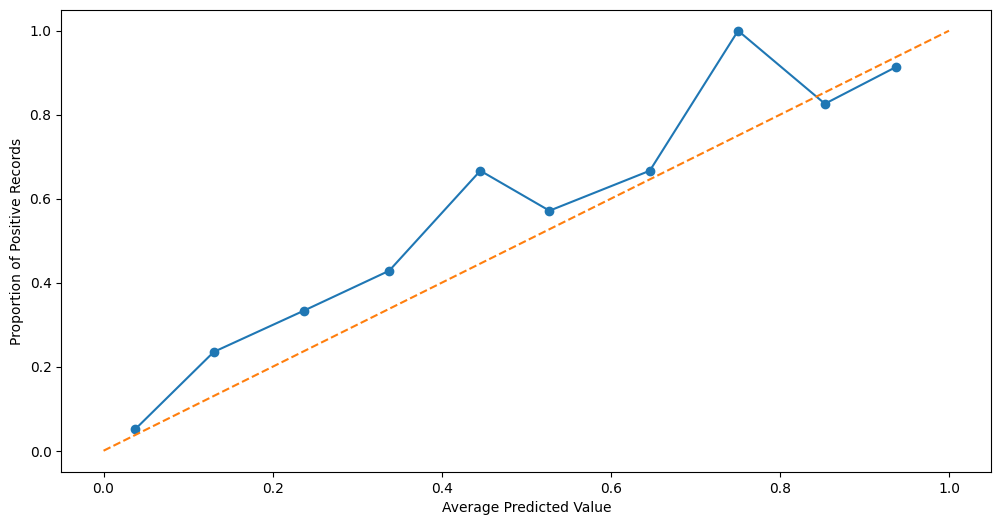}
  \caption{Reliability Diagram of 15 bins}
  \label{fig:ad-15-tc}
\end{subfigure} 
\begin{subfigure}{0.33\textwidth}
  \includegraphics[width=\linewidth]{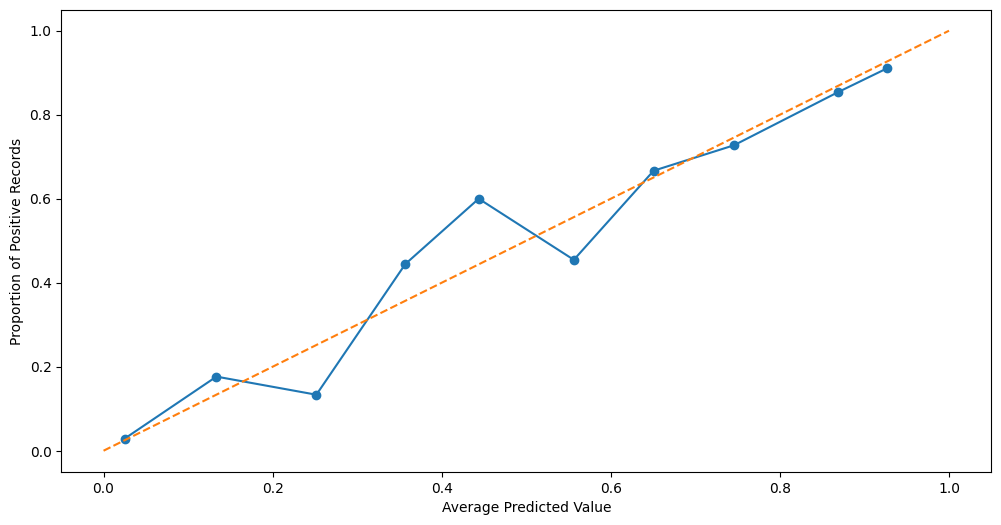}
  \caption{Reliability Diagram of 20 bins}
  \label{fig:ad-20-tc}
\end{subfigure} 
\label{fig:tc-ad}
\caption{Reliability diagrams with synthetic data added on (synthesis+)}
\end{figure}

\endgroup

\clearpage

SUBJ dataset

\begingroup
\setlength{\textfloatsep}{10pt} % Adjust the value as needed

\begin{figure}[h]
\centering
\includegraphics[width=0.5\textwidth]{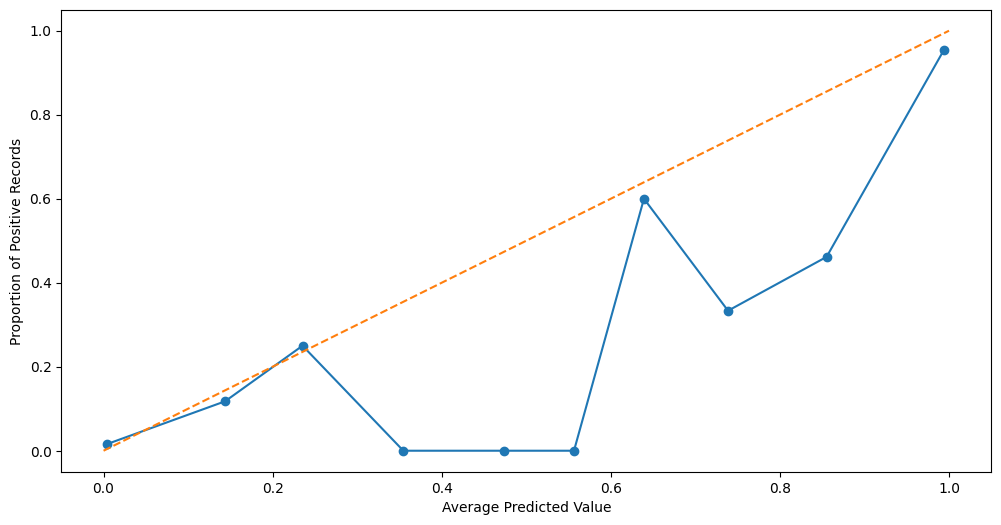}
\caption{\label{fig:bs-sj} The baseline reliability diagram for SUBJ dataset}  
\end{figure}

% \vspace{-10pt} % Adjust the value as needed
\begin{figure}[h]
\begin{subfigure}{0.33\textwidth}
  \includegraphics[width=\linewidth]{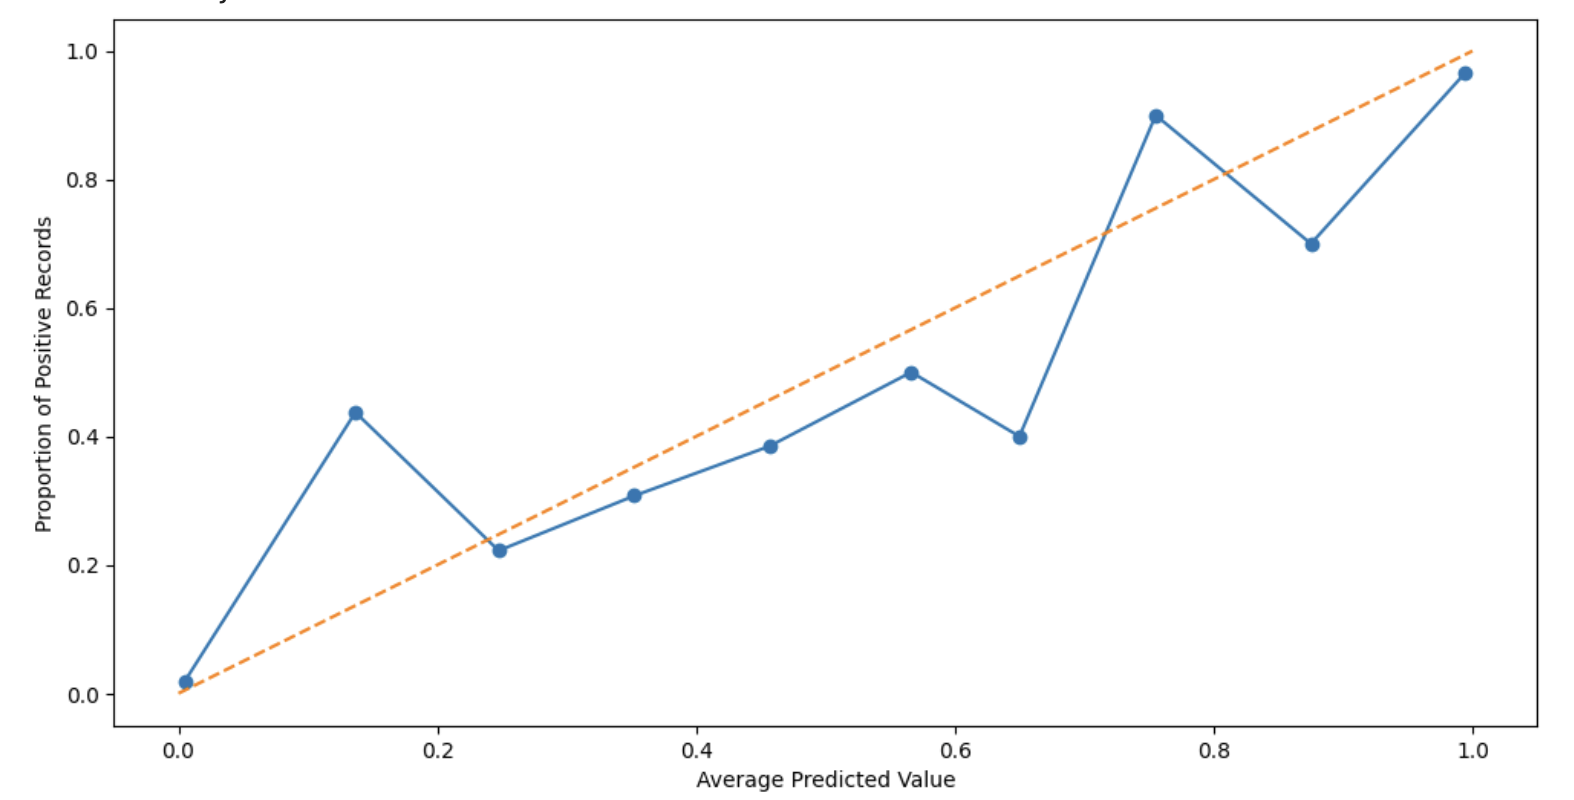}
  \caption{Reliability Diagram of 10 bins}
  \label{fig:rp-10-sj}
\end{subfigure}
\begin{subfigure}{0.33\textwidth}
  \includegraphics[width=\linewidth]{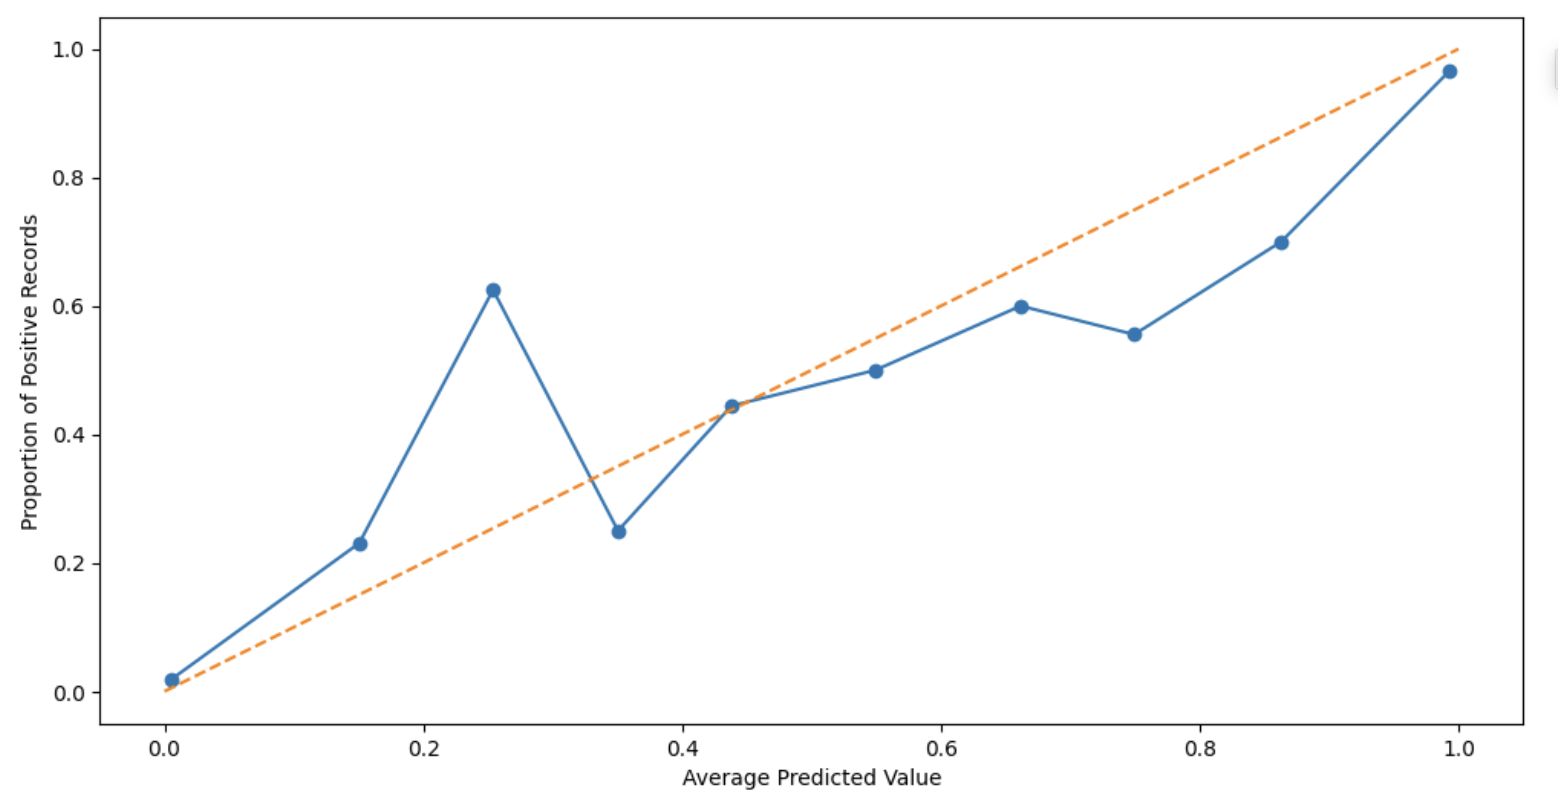}
  \caption{Reliability Diagram of 15 bins}
  \label{fig:rp-15-sj}
\end{subfigure} 
\begin{subfigure}{0.33\textwidth}
  \includegraphics[width=\linewidth]{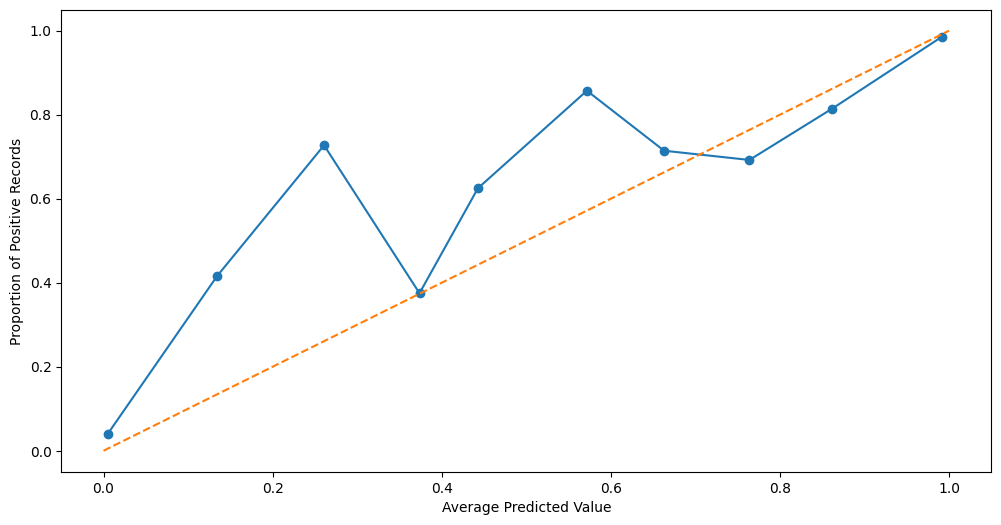}
  \caption{Reliability Diagram of 20 bins}
  \label{fig:rp-20-sj}
\end{subfigure} 
\label{fig:sj-rp}
\caption{Reliability diagrams with synthetic data replacement (synthesis)}
\end{figure}

% \vspace{-50pt} % Adjust the value as needed

\begin{figure}[h]
\begin{subfigure}{0.33\textwidth}
  \includegraphics[width=\linewidth]{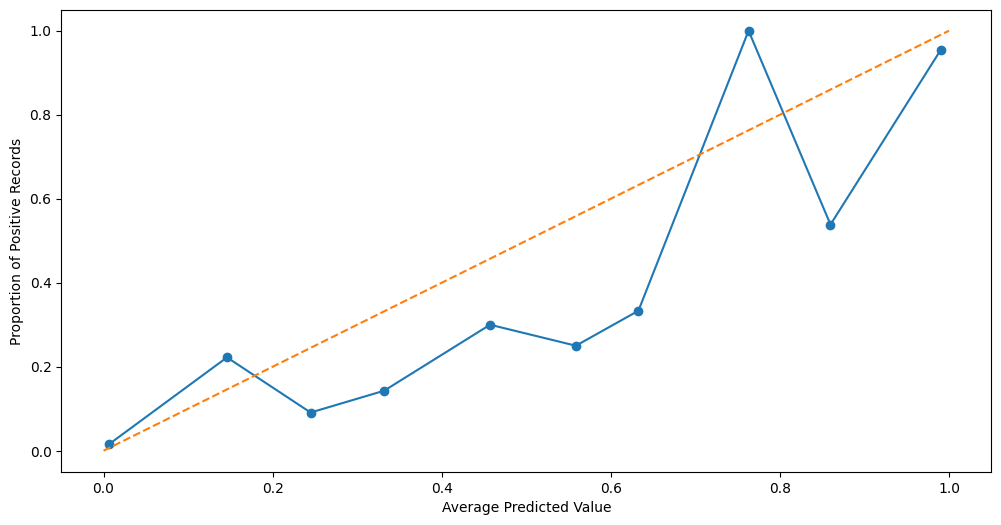}
  \caption{Reliability Diagram of 10 bins}
  \label{fig:ad-10-sj}
\end{subfigure}
\begin{subfigure}{0.33\textwidth}
  \includegraphics[width=\linewidth]{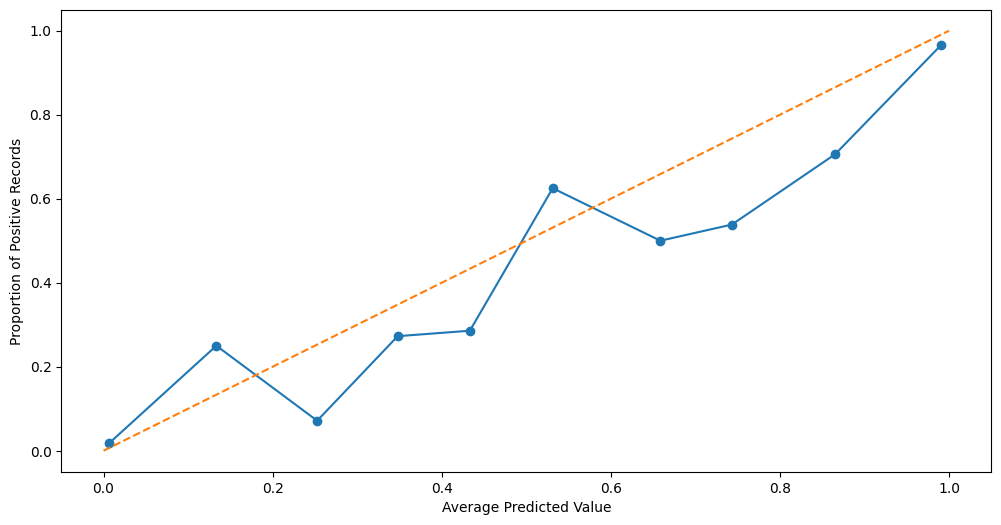}
  \caption{Reliability Diagram of 15 bins}
  \label{fig:ad-15-sj}
\end{subfigure} 
\begin{subfigure}{0.33\textwidth}
  \includegraphics[width=\linewidth]{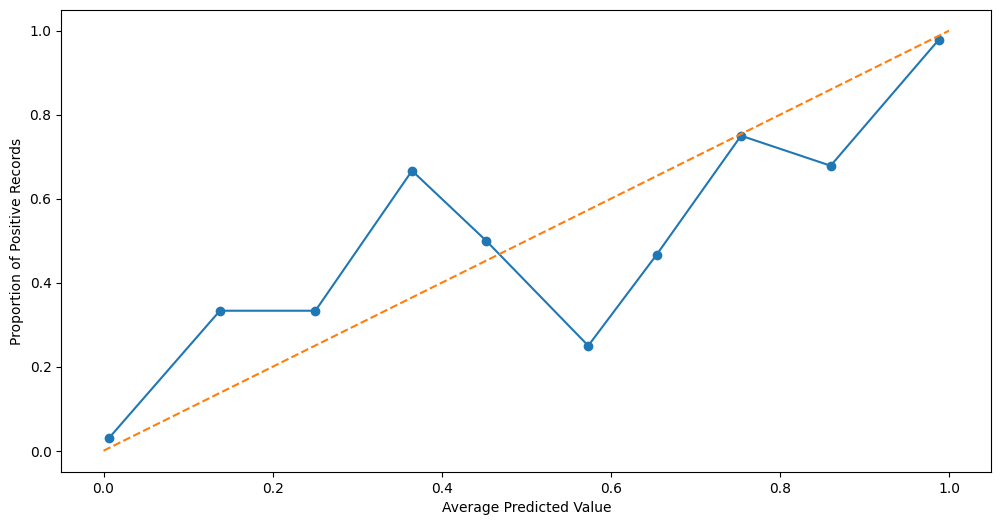}
  \caption{Reliability Diagram of 20 bins}
  \label{fig:ad-20-sj}
\end{subfigure} 
\label{fig:sj-ad}
\caption{Reliability diagrams with synthetic data added on (synthesis+)}
\end{figure}

\endgroup

\clearpage

B77 dataset

\begingroup
\setlength{\textfloatsep}{10pt} % Adjust the value as needed

\begin{figure}[h]
\centering
\includegraphics[width=0.5\textwidth]{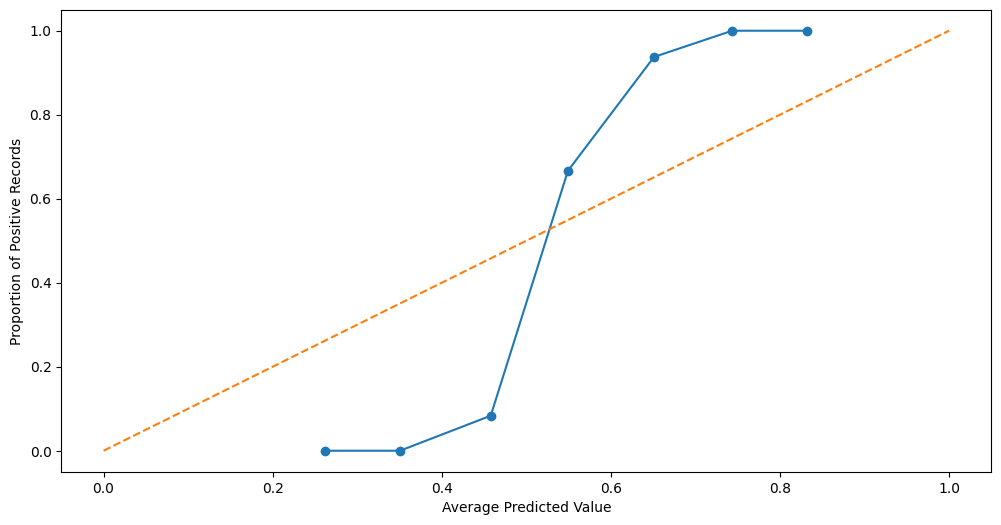}
\caption{\label{fig:bs-b77j} The baseline reliability diagram for SUBJ dataset}  
\end{figure}

% \vspace{-10pt} % Adjust the value as needed
\begin{figure}[h]
\begin{subfigure}{0.33\textwidth}
  \includegraphics[width=\linewidth]{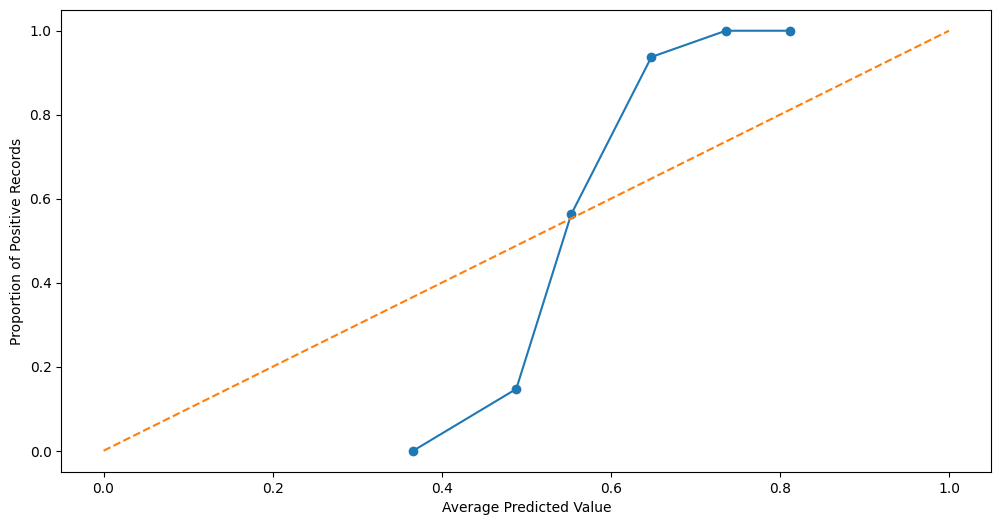}
  \caption{Reliability Diagram of 10 bins}
  \label{fig:rp-10-b77}
\end{subfigure}
\begin{subfigure}{0.33\textwidth}
  \includegraphics[width=\linewidth]{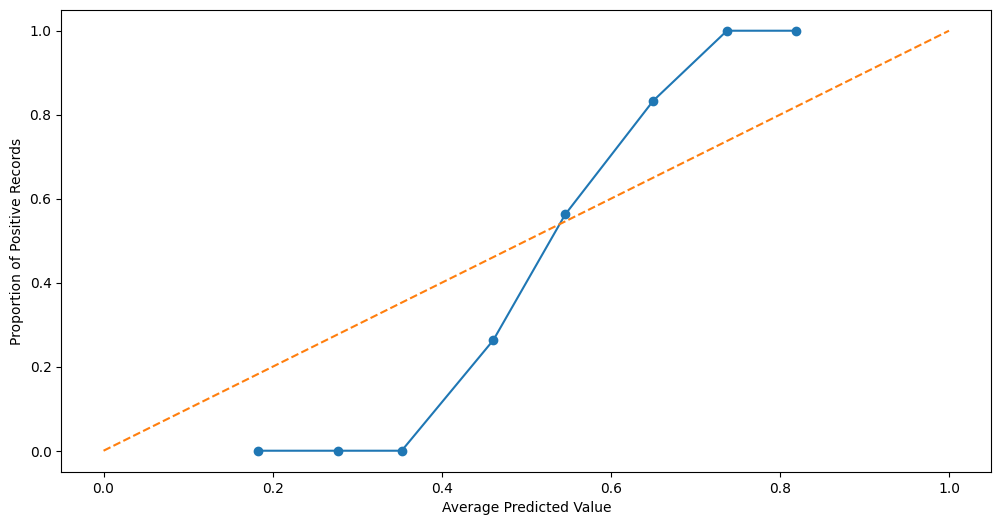}
  \caption{Reliability Diagram of 15 bins}
  \label{fig:rp-15-b77}
\end{subfigure} 
\begin{subfigure}{0.33\textwidth}
  \includegraphics[width=\linewidth]{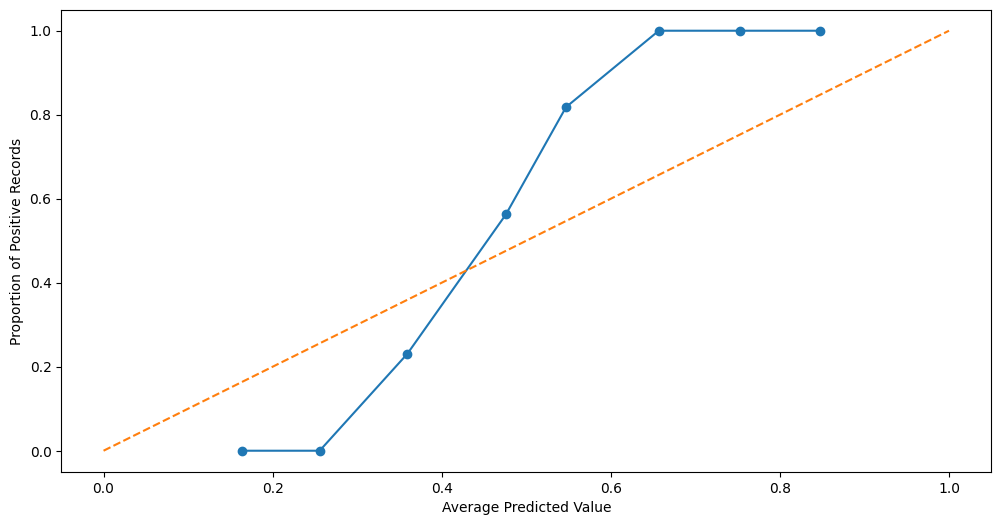}
  \caption{Reliability Diagram of 20 bins}
  \label{fig:rp-20-b77}
\end{subfigure} 
\label{fig:b77-rp}
\caption{Reliability diagrams with synthetic data replacement (synthesis)}
\end{figure}

% \vspace{-50pt} % Adjust the value as needed

\begin{figure}[h]
\begin{subfigure}{0.33\textwidth}
  \includegraphics[width=\linewidth]{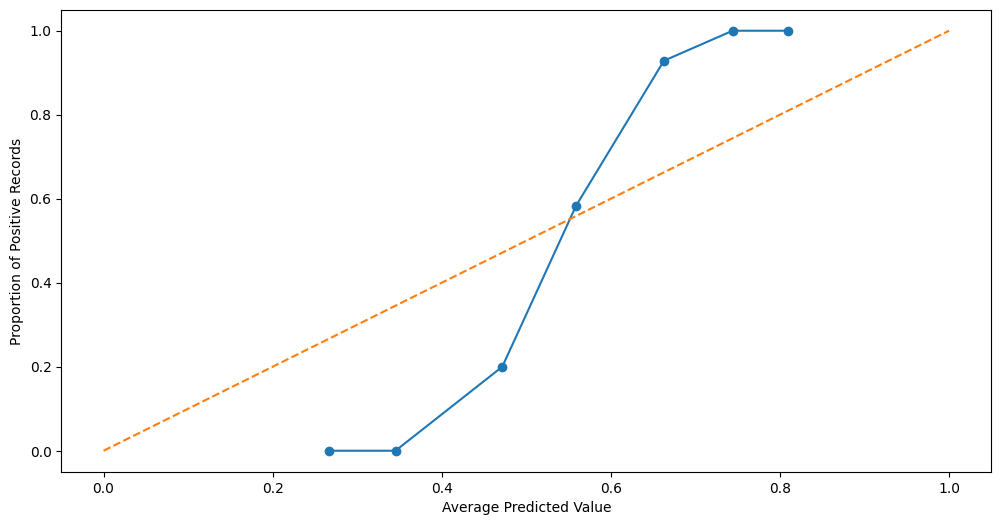}
  \caption{Reliability Diagram of 10 bins}
  \label{fig:ad-10-b77}
\end{subfigure}
\begin{subfigure}{0.33\textwidth}
  \includegraphics[width=\linewidth]{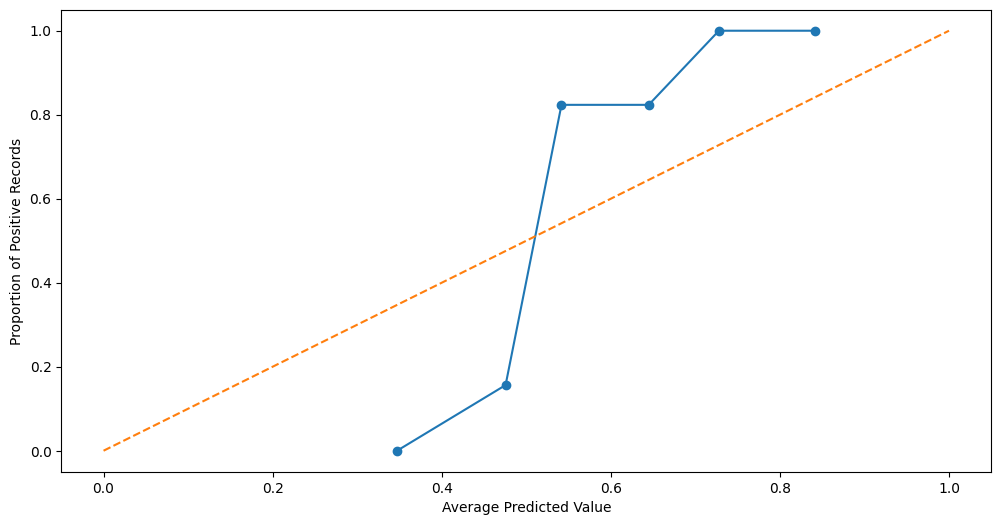}
  \caption{Reliability Diagram of 15 bins}
  \label{fig:ad-15-b77}
\end{subfigure} 
\begin{subfigure}{0.33\textwidth}
  \includegraphics[width=\linewidth]{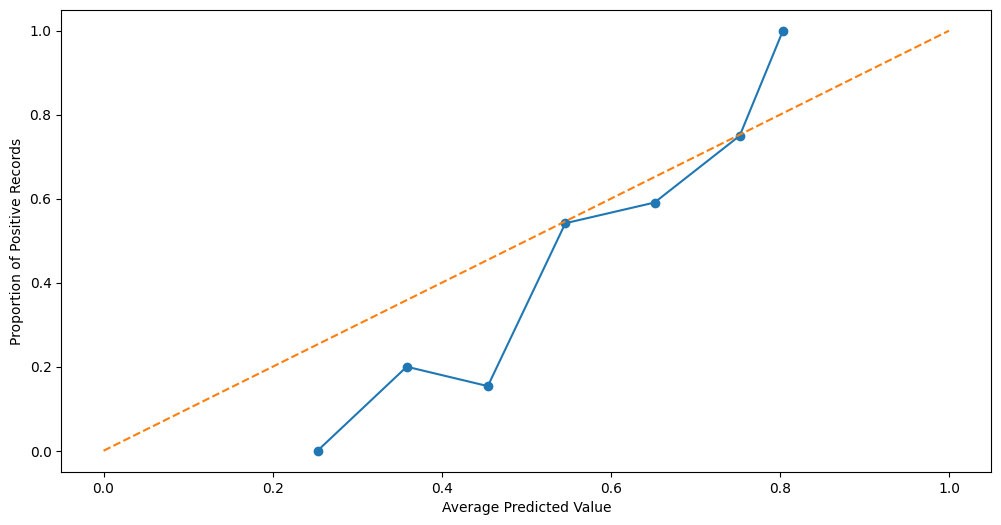}
  \caption{Reliability Diagram of 20 bins}
  \label{fig:ad-20-b77}
\end{subfigure} 
\label{fig:b77-ad}
\caption{Reliability diagrams with synthetic data added on (synthesis+)}
\end{figure}

\endgroup

\clearpage
SE dataset: 

\begingroup
\setlength{\textfloatsep}{10pt} % Adjust the value as needed

\begin{figure}[h]
\centering
\includegraphics[width=0.5\textwidth]{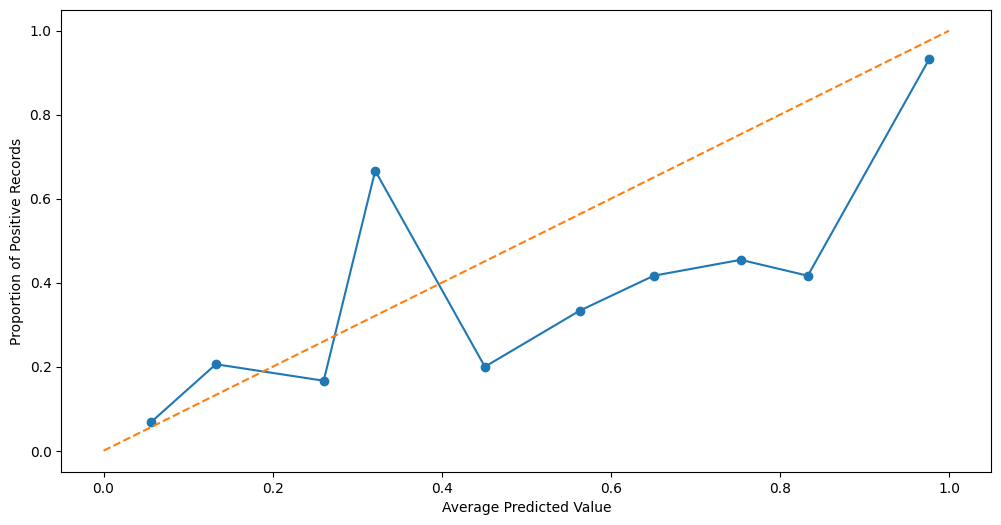}
\caption{\label{fig:bs-se} The baseline reliability diagram for SE dataset}  
\end{figure}

% \vspace{-10pt} % Adjust the value as needed
\begin{figure}[h]
\begin{subfigure}{0.33\textwidth}
  \includegraphics[width=\linewidth]{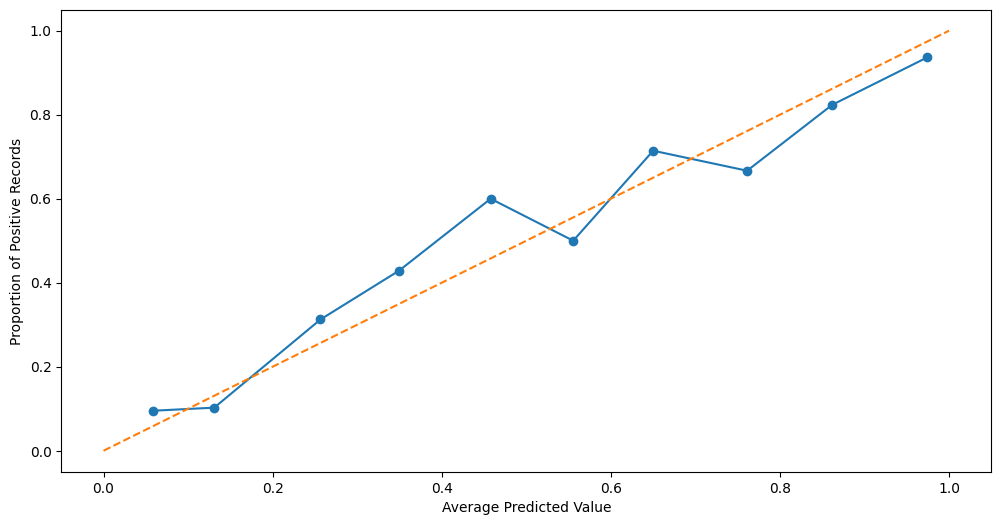}
  \caption{Reliability Diagram of 10 bins}
  \label{fig:rp-10-se}
\end{subfigure}
\begin{subfigure}{0.33\textwidth}
  \includegraphics[width=\linewidth]{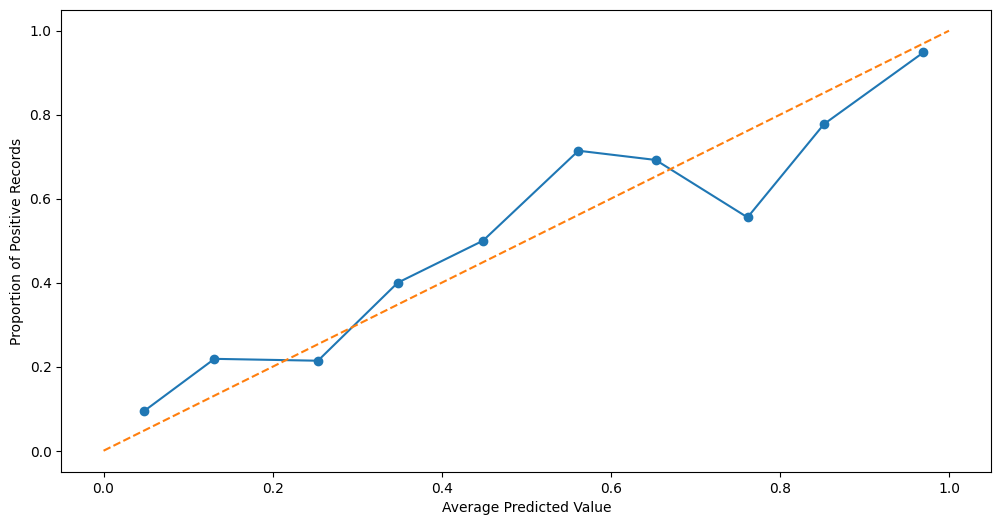}
  \caption{Reliability Diagram of 15 bins}
  \label{fig:rp-15-se}
\end{subfigure} 
\begin{subfigure}{0.33\textwidth}
  \includegraphics[width=\linewidth]{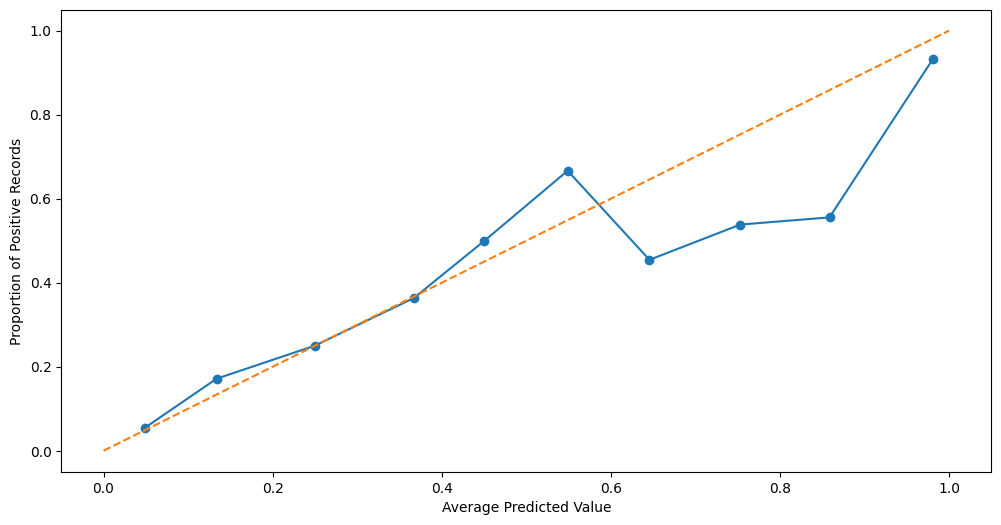}
  \caption{Reliability Diagram of 20 bins}
  \label{fig:rp-20-se}
\end{subfigure} 
\label{fig:se-rp}
\caption{Reliability diagrams with synthetic data replacement (synthesis)}
\end{figure}

% \vspace{-50pt} % Adjust the value as needed

\begin{figure}[h]
\begin{subfigure}{0.33\textwidth}
  \includegraphics[width=\linewidth]{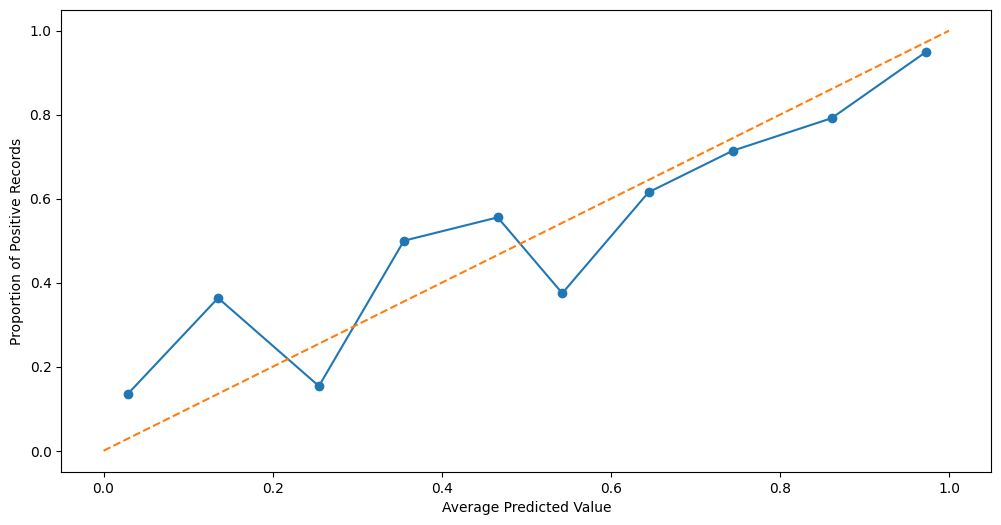}
  \caption{Reliability Diagram of 10 bins}
  \label{fig:ad-10-se}
\end{subfigure}
\begin{subfigure}{0.33\textwidth}
  \includegraphics[width=\linewidth]{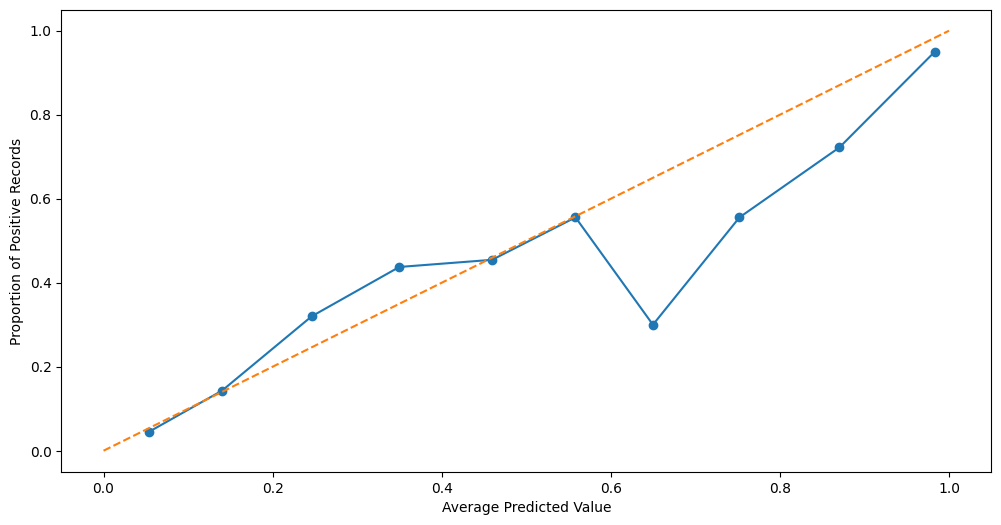}
  \caption{Reliability Diagram of 15 bins}
  \label{fig:ad-15-se}
\end{subfigure} 
\begin{subfigure}{0.33\textwidth}
  \includegraphics[width=\linewidth]{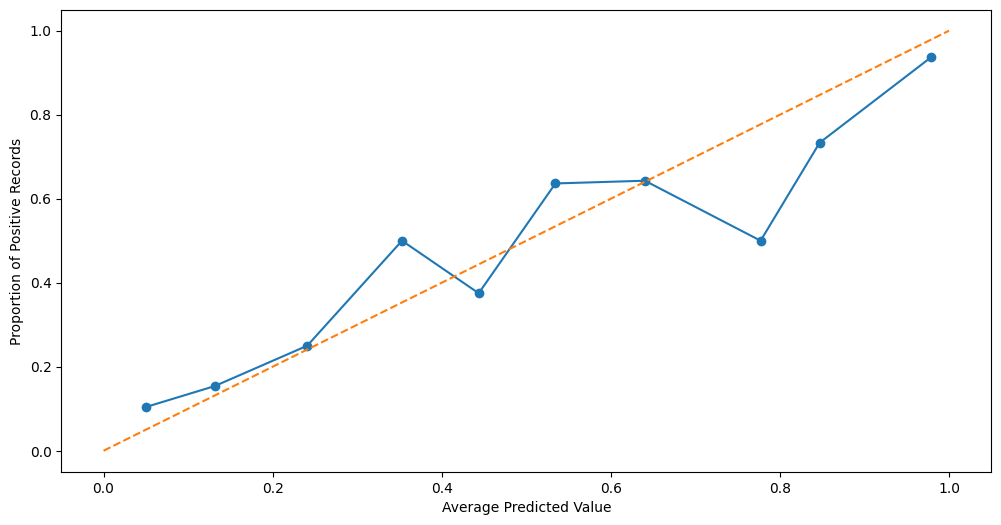}
  \caption{Reliability Diagram of 20 bins}
  \label{fig:ad-20-se}
\end{subfigure} 
\label{fig:se-ad}
\caption{Reliability diagrams with synthetic data added on (synthesis+)}
\end{figure}

\endgroup

\clearpage
